# Supplementary material for: Dynamic Visual Semantic Sub-Embeddings and Fast Re-Ranking
Source: arXiv:2309.08154 source file (2023-12-21)
Supplement: Supplementary file 1 [file X_suppl.tex]

\clearpage
\setcounter{page}{1}
\maketitlesupplementary

\section{Experiments}
% 在本节，我们将介绍本文具体的实验细节以及数据集和评价指标的选择。
\subsection{Datasets and Metrics} 
\subsubsection{Datasets}
\textbf{MSCOCO} consists of 123,287 images and 616,435 textual descriptions. We followed the same splits [8], which allocated 5,000 images for validation, 5,000 images for testing, and 113,287 images for training. We evaluated our model in two settings within MS-COCO: 1) 1K Test, which combines results from five sets of 1K test images, and 2) 5K Test, which involves testing on the entire 5K test images.

\noindent
\textbf{Flickr30K} consists of 31,783 images and 158,915 sentence descriptions. It follows the data splits [8], where 1,000 images were set aside for testing, another 1,000 for validation, and the rest were used for training.

\noindent
\textbf{CUB Captions} encompasses 11,788 images in 200 fine-grained bird categories, each accompanied by 10 captions. We adhered to the class splits defined in [50], which allocated 150 classes for training and validation, reserving the remaining 50 for testing. Given the homogeneous nature of images and texts within the same class, this dataset effectively mitigates false positives.

\subsubsection{Evaluation Metrics.} 
To assess our model's performance, we utilized the Recall@K metric to measure retrieval accuracy and the RP and PMRP metrics to quantify retrieval diversity.

\noindent
\textbf{Recall@K (R@K)}
Recall@K measures the percentage of test samples where the correct match appears in the top K retrieved results. Specifically, for both the image retrieval and text retrieval, we used Recall@1, Recall@5, and Recall@10 to measure the accuracy of our model, respectively.

\noindent
\textbf{R-Precision (R-P)}
R-Precision is an evaluation metric that considers the order of rankings. It assesses how many of the top R results returned are pertinent to the query, making it more suitable for gauging the diversity of the model.

\noindent
\textbf{Plausible Match R-Precision (PMRP)}
PMRP measures whether a pair $i,c$ is declared positive if the binary label vectors for the two instances, $y^i,y^c \in \{0,1\}^{d^{label}}$, differ at most at $\zeta$ positions. Therefore, it can be used to search for further credible positive matches in the database by considering additional information.

\subsection{Implementation Details}
% 本文所有的实验都使用PyTorch  1.11.0，初始学习率都设置为0.0005.
\noindent
\textbf{ResNet-152 + Bi-GRU}

\noindent
\textbf{Faster R-CNN + Bi-GRU}

\noindent
\textbf{ResNeXt-101 + BERT}

\noindent
\textbf{ResNet-50 + Bi-GRU}

\section{Fast Re-ranking}

% 
% Having the supplementary compiled together with the main paper means that:
% % 
% \begin{itemize}
% \item The supplementary can back-reference sections of the main paper, for example, we can refer to \cref{sec:intro};
% \item The main paper can forward reference sub-sections within the supplementary explicitly (e.g. referring to a particular experiment); 
% \item When submitted to arXiv, the supplementary will already included at the end of the paper.
% \subsubsection{Effects of different configurations of hyper-parameters}

% % \subsubsection{Bounding representations of cross-modal consistency constraints}
% % \input{table/diversity and accuracy}

% \end{itemize}
% % 
% To split the supplementary pages from the main paper, you can use \href{https://support.apple.com/en-ca/guide/preview/prvw11793/mac#:~:text=Delete%20a%20page%20from%20a,or%20choose%20Edit%20%3E%20Delete).}{Preview (on macOS)}, \href{https://www.adobe.com/acrobat/how-to/delete-pages-from-pdf.html#:~:text=Choose%20%E2%80%9CTools%E2%80%9D%20%3E%20%E2%80%9COrganize,or%20pages%20from%20the%20file.}{Adobe Acrobat} (on all OSs), as well as \href{https://superuser.com/questions/517986/is-it-possible-to-delete-some-pages-of-a-pdf-document}{command line tools}.
